# Supplementary material for: Efficient Full Image Interactive Segmentation by Leveraging Within-image Appearance Similarity
Source: arXiv:2007.08173 source file (2020-07-16)
Supplement: Supplementary file 1 [file appendix.tex]

\appendix

\section{Evaluation Details}
\begin{figure}[t]
\begin{center}
\begin{tabular}{ccc}
  \includegraphics[width=0.33\linewidth]{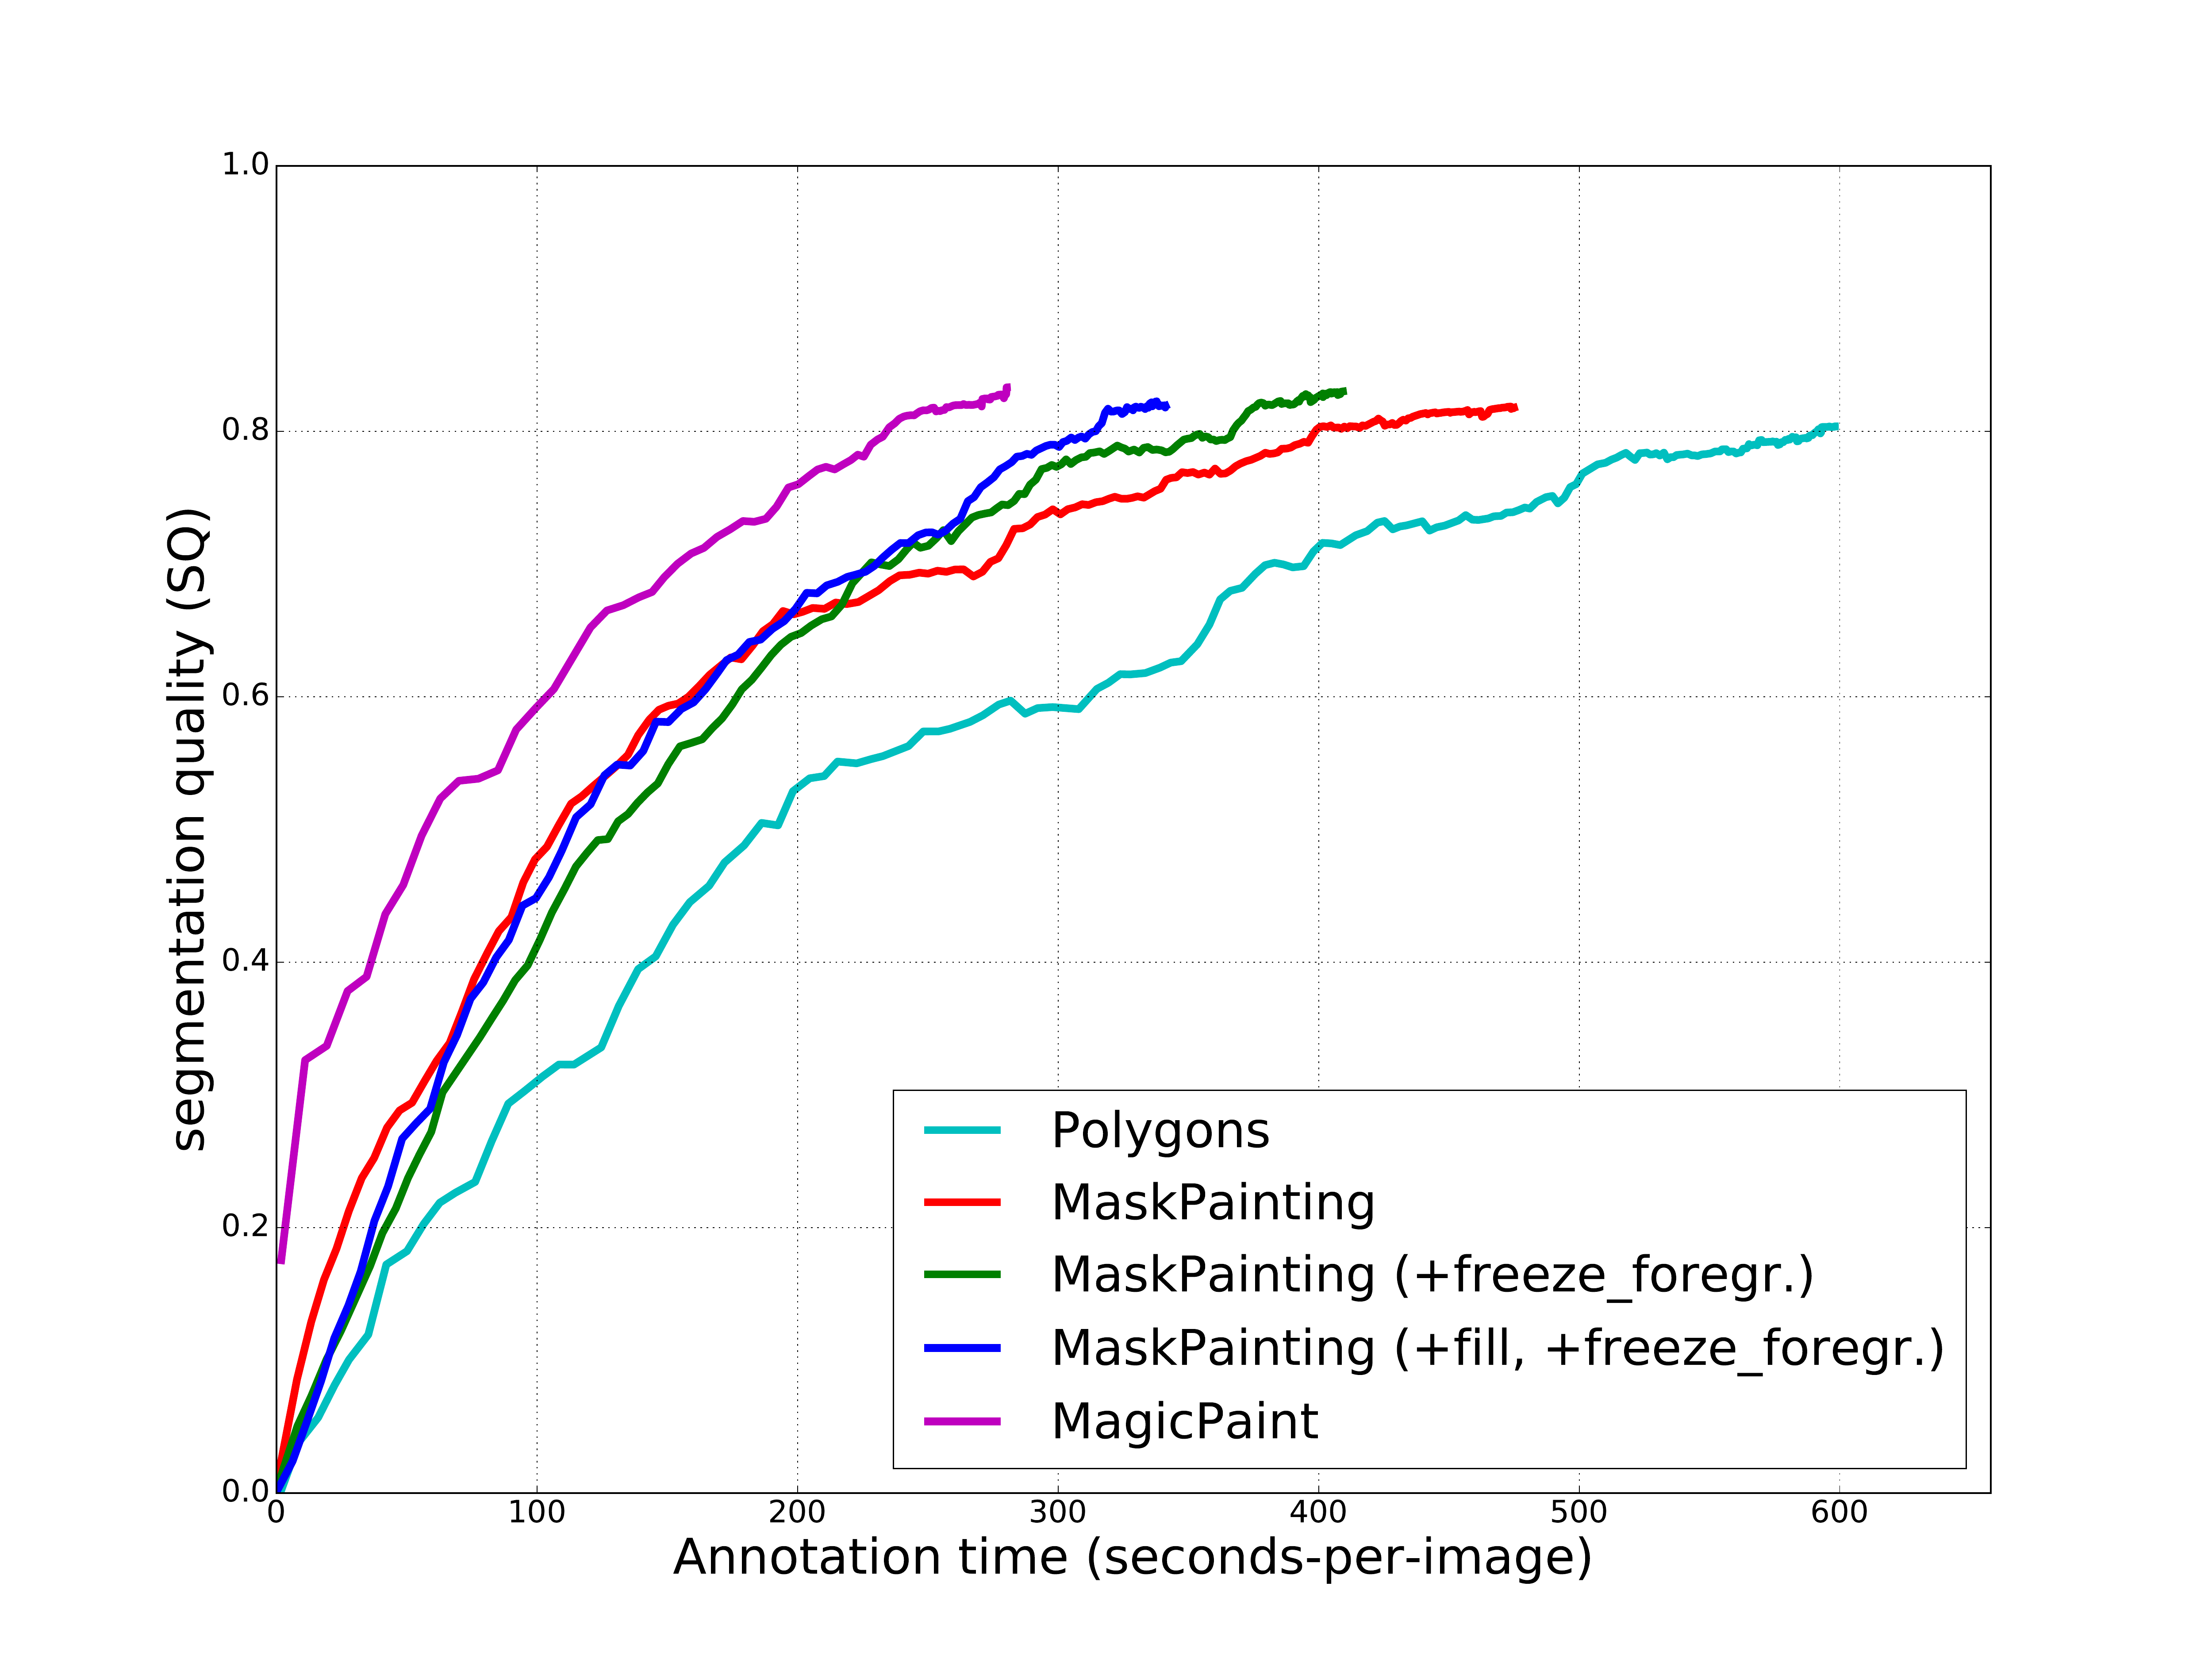}&
  \includegraphics[width=0.33\linewidth]{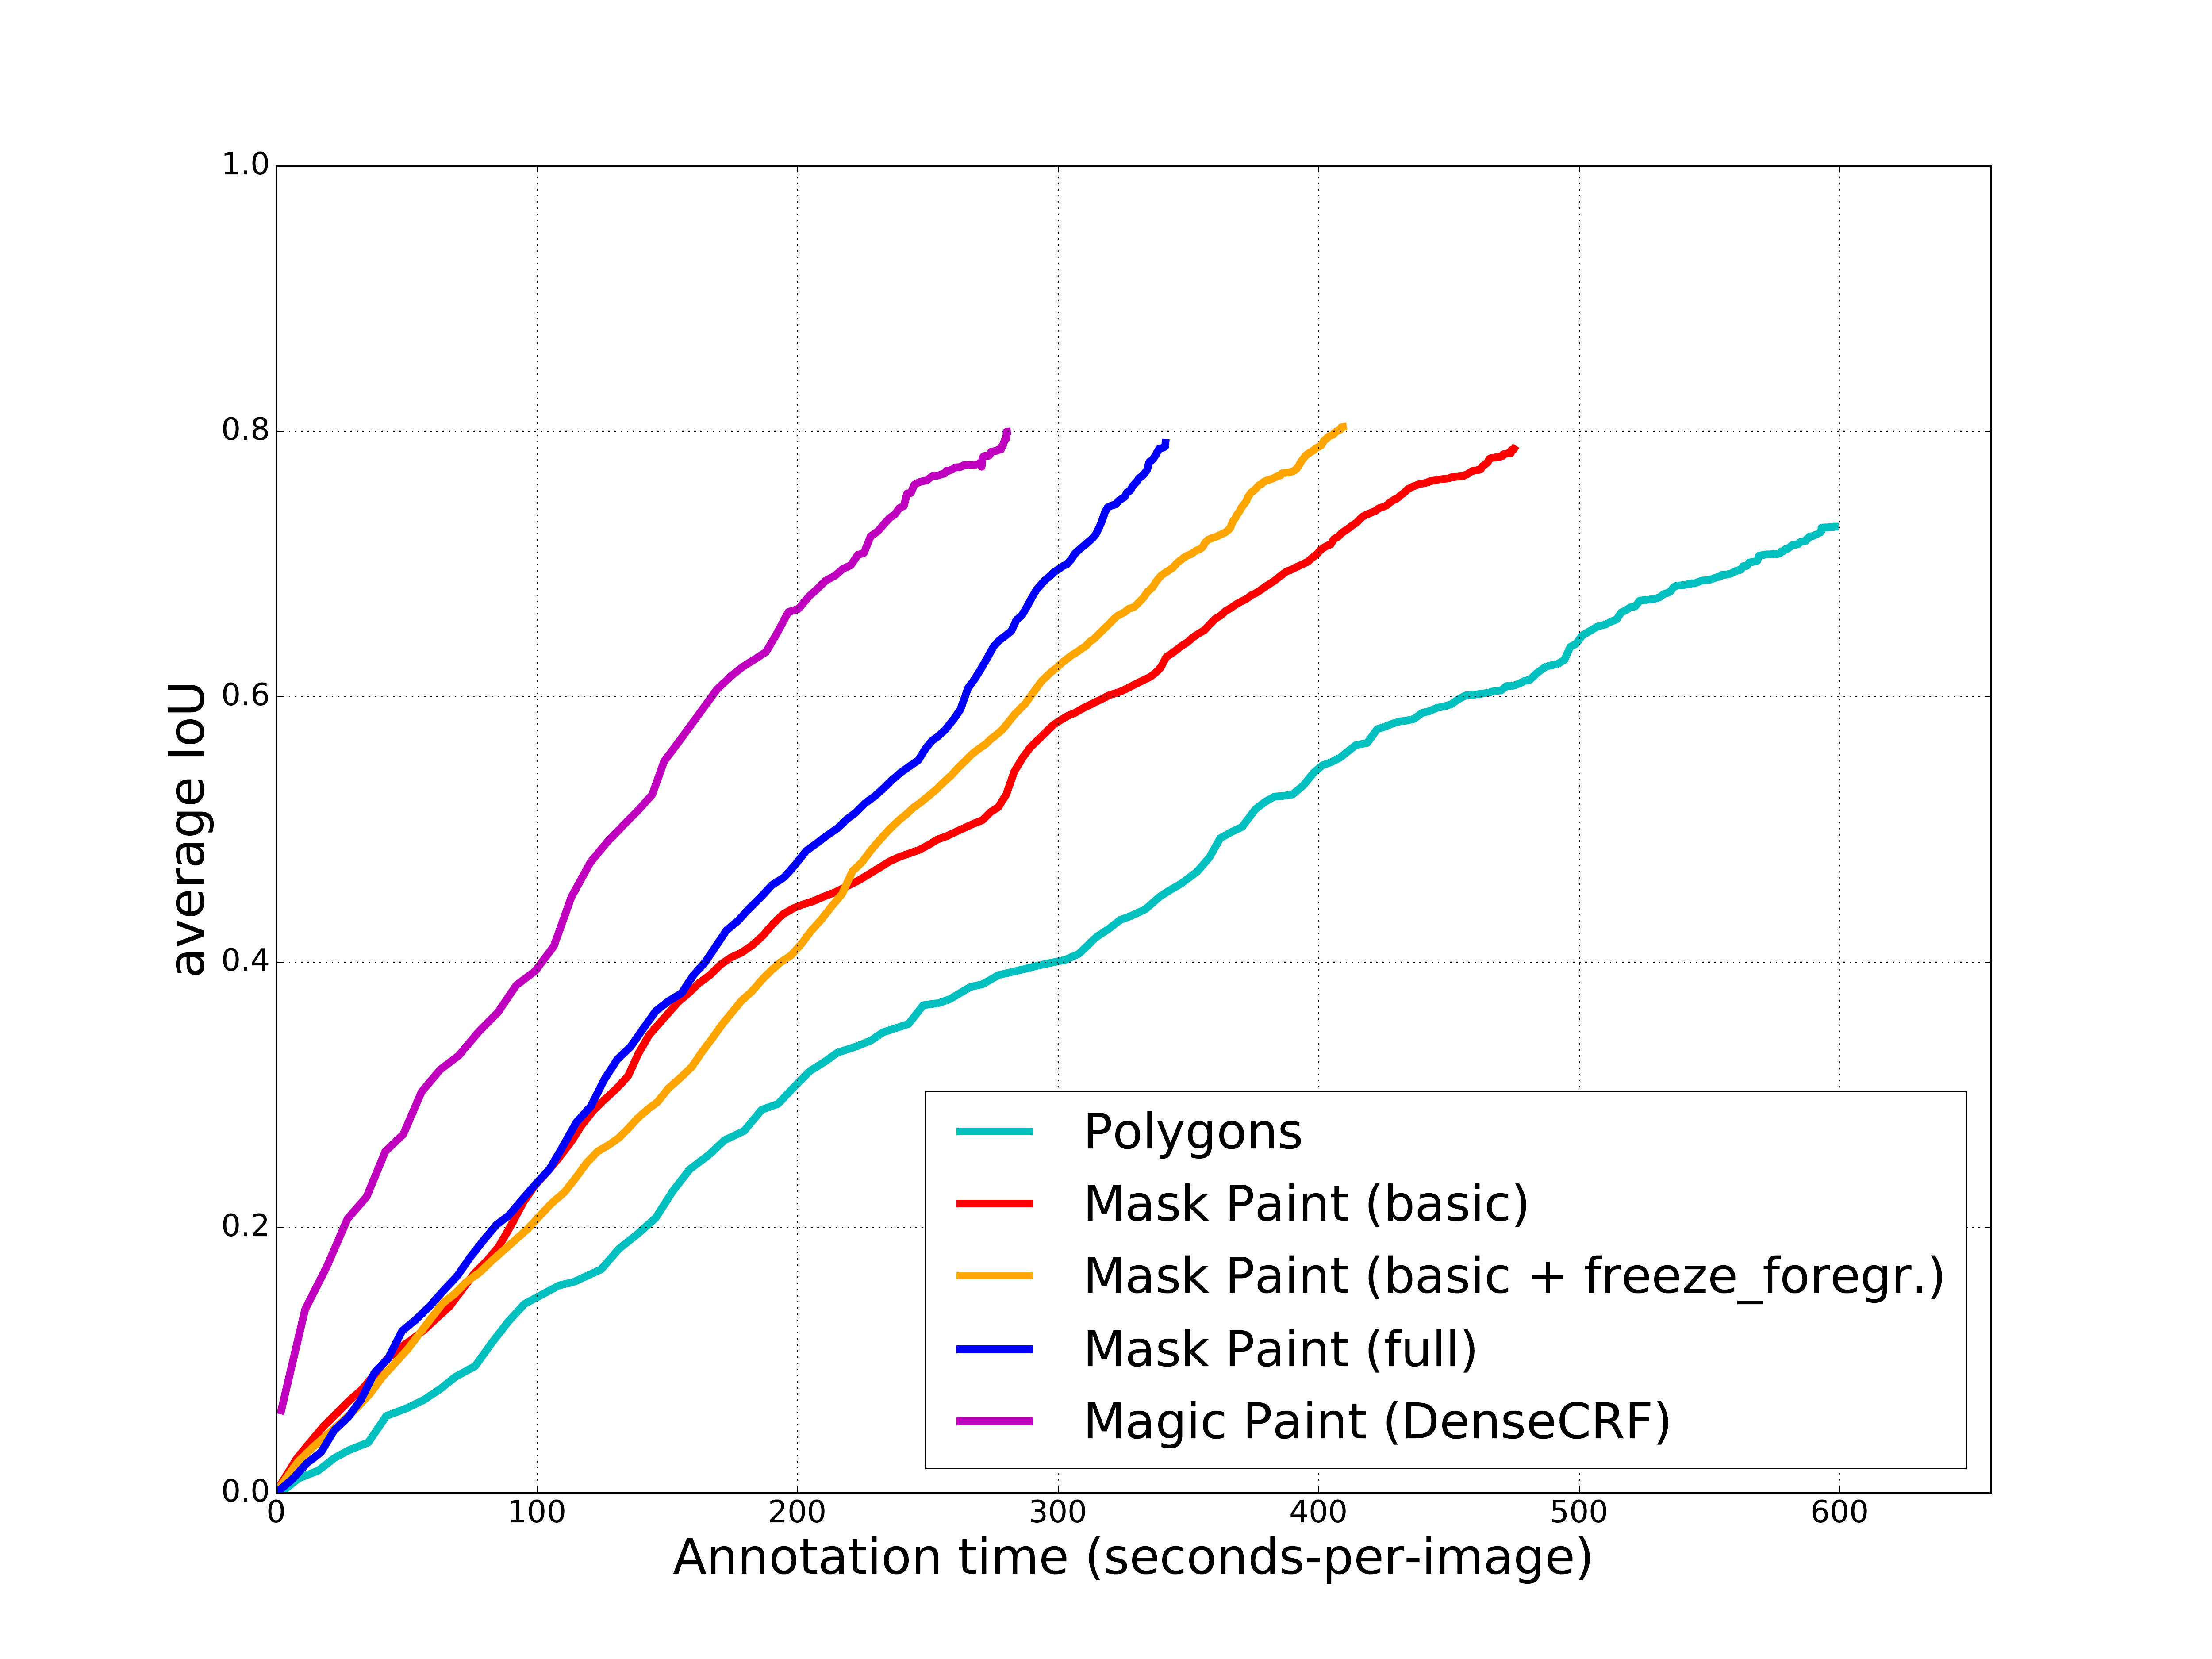}&
  \includegraphics[width=0.33\linewidth]{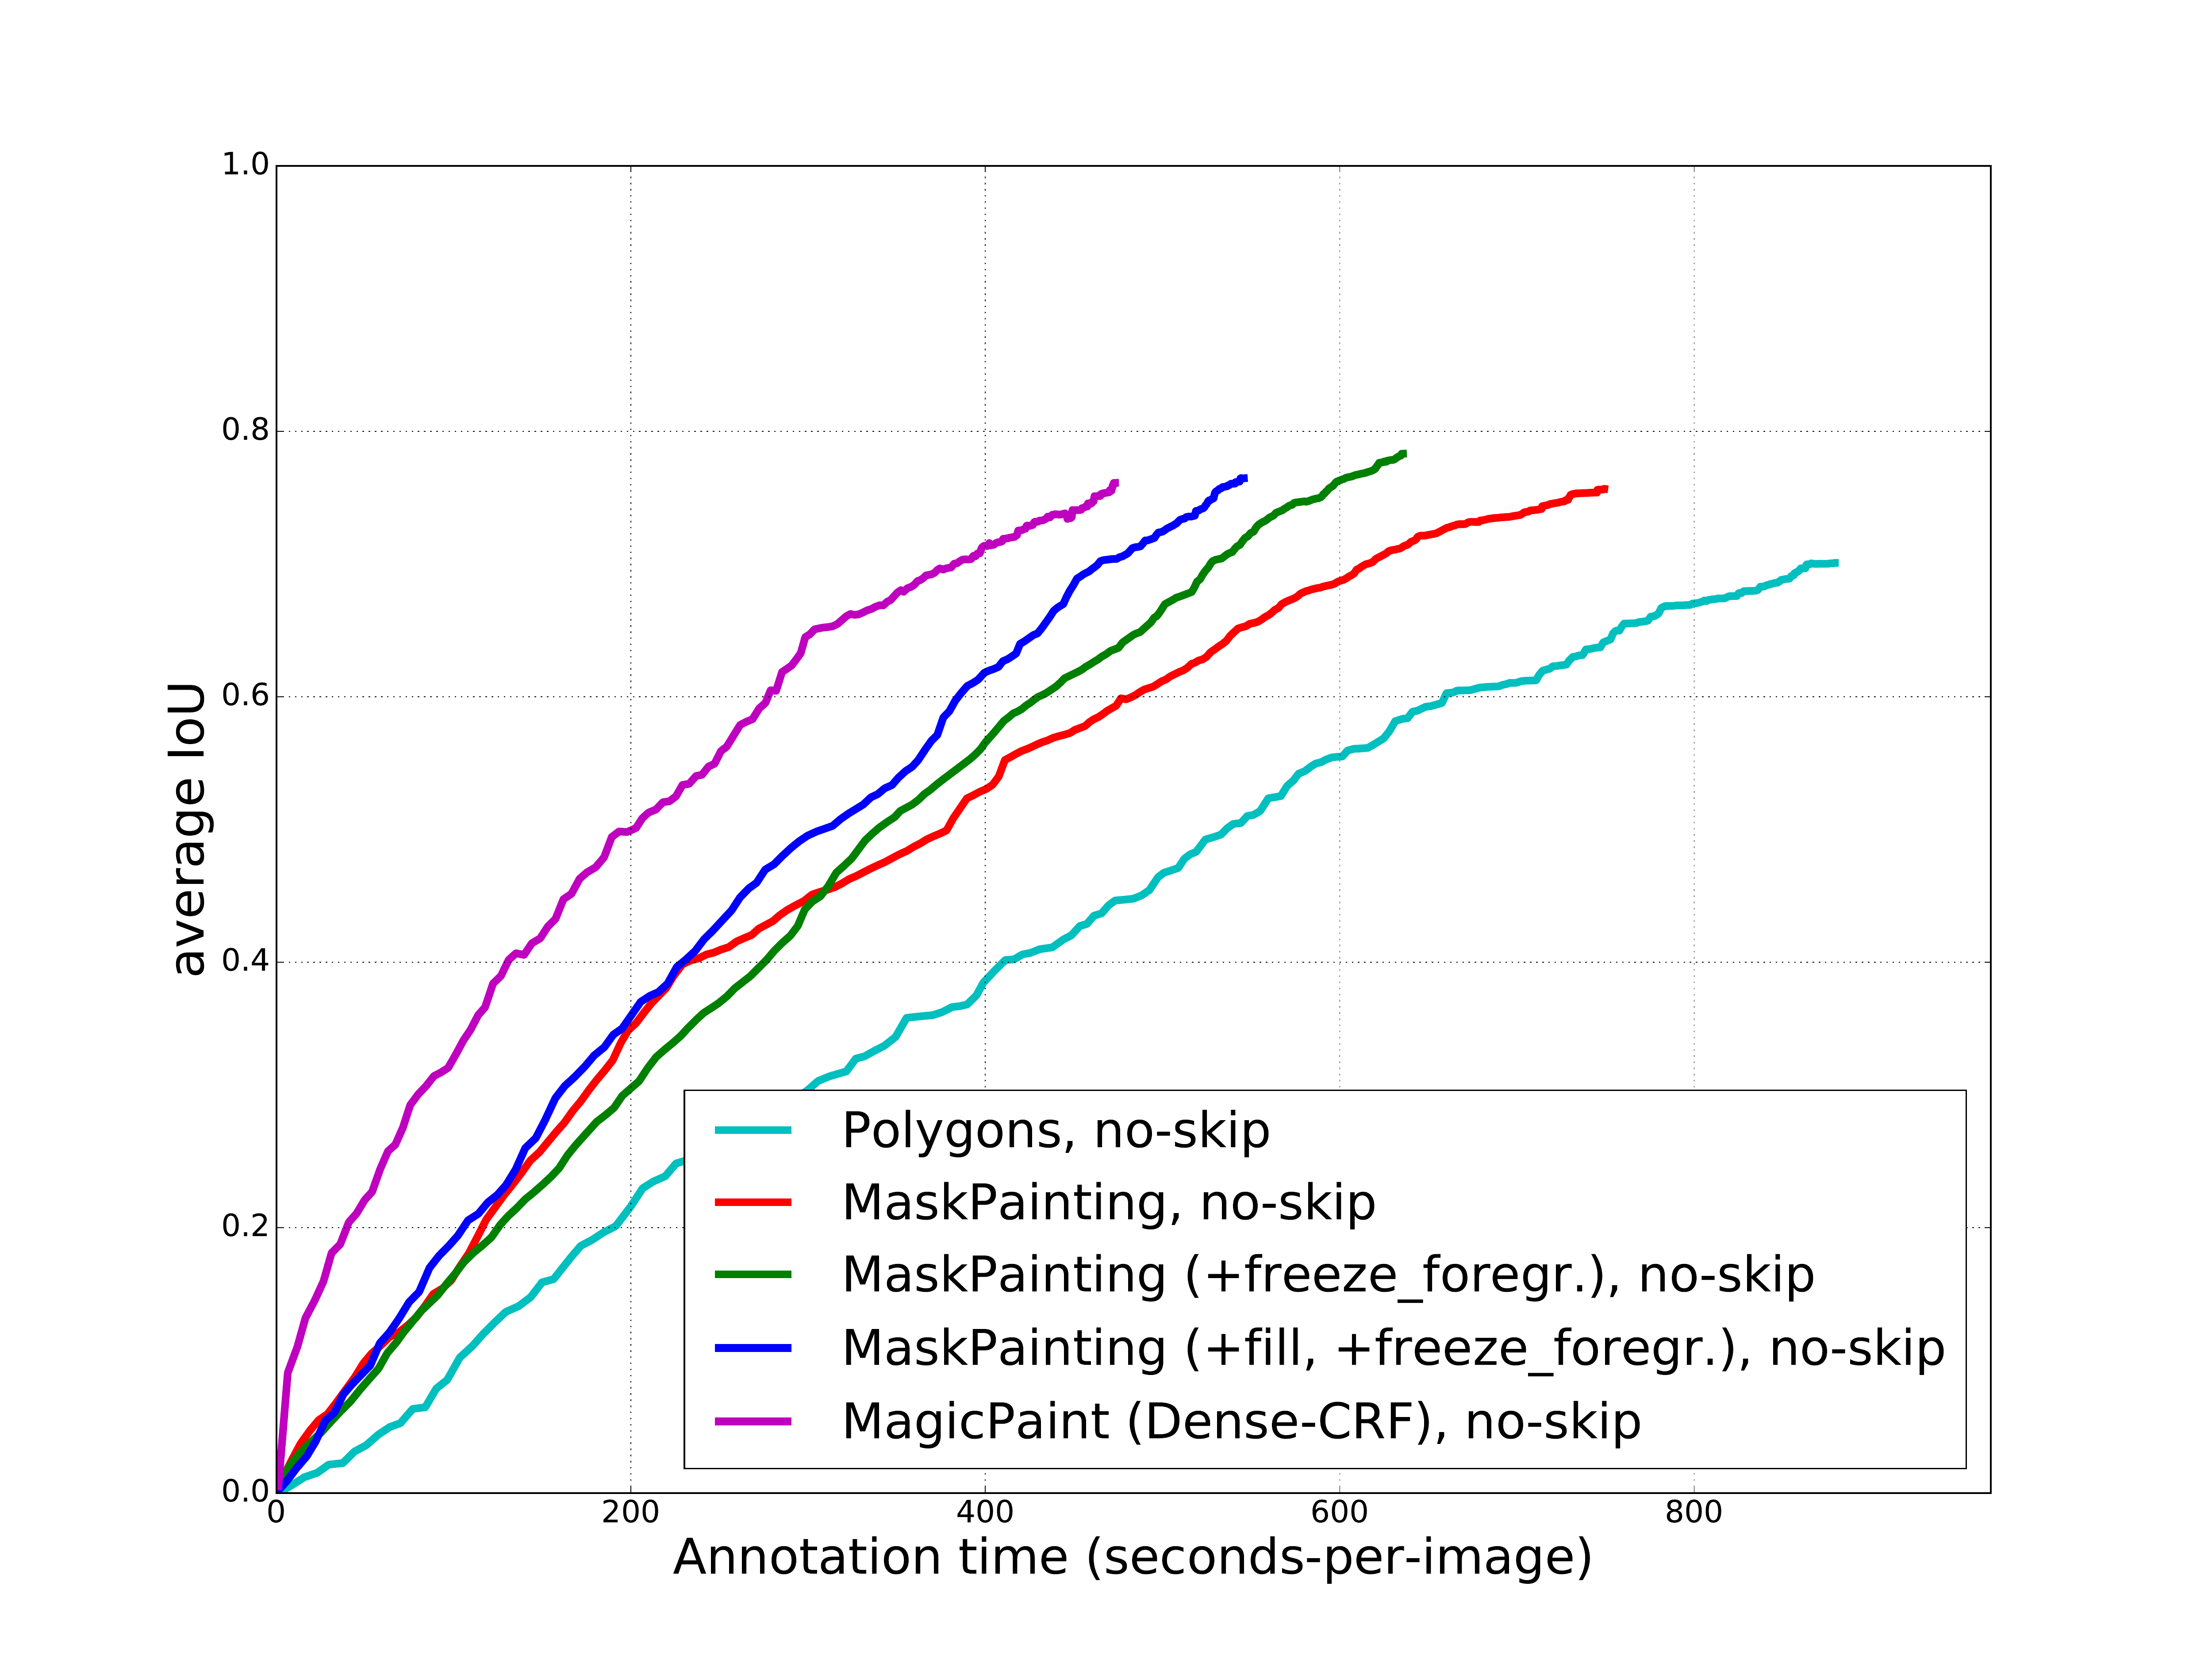}\\
(a) & (b) & (c)\\
\end{tabular}
\end{center}
\caption{Additional evaluation results on the COCO-val100 dataset. We compare evaluation results using segmentation quality (a) and average IoU (b). The plot in (c) shows evaluation without skipping redundant annotation actions. Note that the MagicPaint plots shown in (a) and (b) are the best-case plots that assume that predictions are available immediately.}
\label{fig:eval_appendix}
\end{figure}
In this section we describe the details of the evaluation protocol used to compare annotation
methods in this paper in Fig.~\ref{fig:eval_coco} and \ref{fig:eval_transfer}. 

\myparagraph{Evaluation metric.} In Fig.~\ref{fig:eval_coco} and \ref{fig:eval_transfer} we compare
annotation methods using curves that plot average IoU (aIoU) with respect to average annotation
time measured. The aIoU in these plots corresponds to segmentation quality (SQ) in the panoptic
quality metric \cite{kirillov19cvpr}\footnote{See Eq.~2 in \cite{kirillov19cvpr}.}:
\begin{equation}
\mbox{SQ} = \frac{\sum_{(p,q) \in TP}\mbox{IoU}(p,q)}{|TP|}, 
\end{equation}
where $(p, q)$ is a pair of matching annotated and ground-truth segments and the matching threshold
to is set to $\tau_{IoU}=0$, which means that the annotated segment is considered to be a true
positive if it has non-zero overlap
with the ground-truth segment. 

Note that the proper aIoU is defined as 
\begin{equation}
\mbox{aIoU} = \frac{\sum_{(p,q) \in TP}\mbox{IoU}(p,q)}{N}, 
\end{equation}
where $N=TP+FN$ is the total number of segments in the ground-truth and we allow at most one match between
annotated and ground-truth segments. Note that in the experiments in this paper we present ground-truth to the
annotator as a reference. This means that with a few exceptions all ground-truth segments will be
annotated so that in the end of the annotation $FN$ should
close to zero and the SQ and aIoU metrics should be equivalent to each other. However the meaning of
the two metrics differs when we evaluate partial annotations as is needed for plotting the annotation progress
vs. time. The SQ measures the quality of the partially
annotated segments, but ignores segments without any annotations. In contrast mIoU considers all of
the segments at all times. Note that yet another variant of aIoU would be to compute averages over annotated
pixels instead of averaging over images, but we do not consider pixel-average aIoU here. We compare evaluations with respect to segmentation quality
(SQ) and aIoU in Fig.~\ref{fig:eval_appendix} (a,b). Note that the shapes of the curves is somewhat
different, but the ordering of the methods is the same. In the end of the aIoU is slightly lower
than SQ indicating that a small number of the ground-truth segments havn't been labeled.

\myparagraph{Thresholding pauses in the annotation logs.} In practice we observe that annotators might take a
longer break during the annotation process \footnote{In some cases we observed pauses that last longer than 1
minute.} and we would like to factor out the effect of such breaks from the evaluation. To that end 
we threshold the maximum pause between annotation actions to a maximum value of 5
seconds. We show the effect of this thresholding in Fig. ~\ref{}.

\myparagraph{Skipping redundant annotation actions.} Recall that some of the experiments in this paper rely on simulation (c.f.~\ref{subsec:simenv}). In
particular our simulation environment skips annotation actions that do not improve the aIoU with
respect to ground-truth. Since annotators do not directly observe the effect of their actions on the
quality metric it is possible that some of their actions do not improve the quality metric. For
example it is possible that annotators aim to generate a particularly clean boundary between object
classes whereas in the ground-truth is annotation is not accurate enough to reward for an extra
precision. In order to make simulated and real annotation evaluations comparable we skip redundant
actions that do not improve annotation quality both for simulated and real annotations. In
Fig.~\ref{fig:eval_appendix}(c) we include evaluation without skipping the redundant actions.

\myparagraph{MagicPaint evaluation.} Our MagicPaint approach typically requires $2$ to $4$ seconds
to generate the prediction. During evaluation we can either directly evaluate the MagicPaint
annotation log or we can simulate the ``best case'' system that would immediately deliver
predictions after each annotation. Note that the ``best case'' system has an advantage that
predictions are available immediately following the input which allows to spare some of the
subsequent annotator actions. We compare the two evaluations in Fig.~\ref{fig:eval_appendix} (b) and
(c).
