# Supplementary material for: Efficient Full Image Interactive Segmentation by Leveraging Within-image Appearance Similarity
Source: arXiv:2007.08173 source file (2020-07-16)
Supplement: Supplementary file 2 [file fig_appendix.tex]

\begin{figure}[t]
\begin{center}
\begin{tabular}{ccc}
  \includegraphics[width=0.33\linewidth]{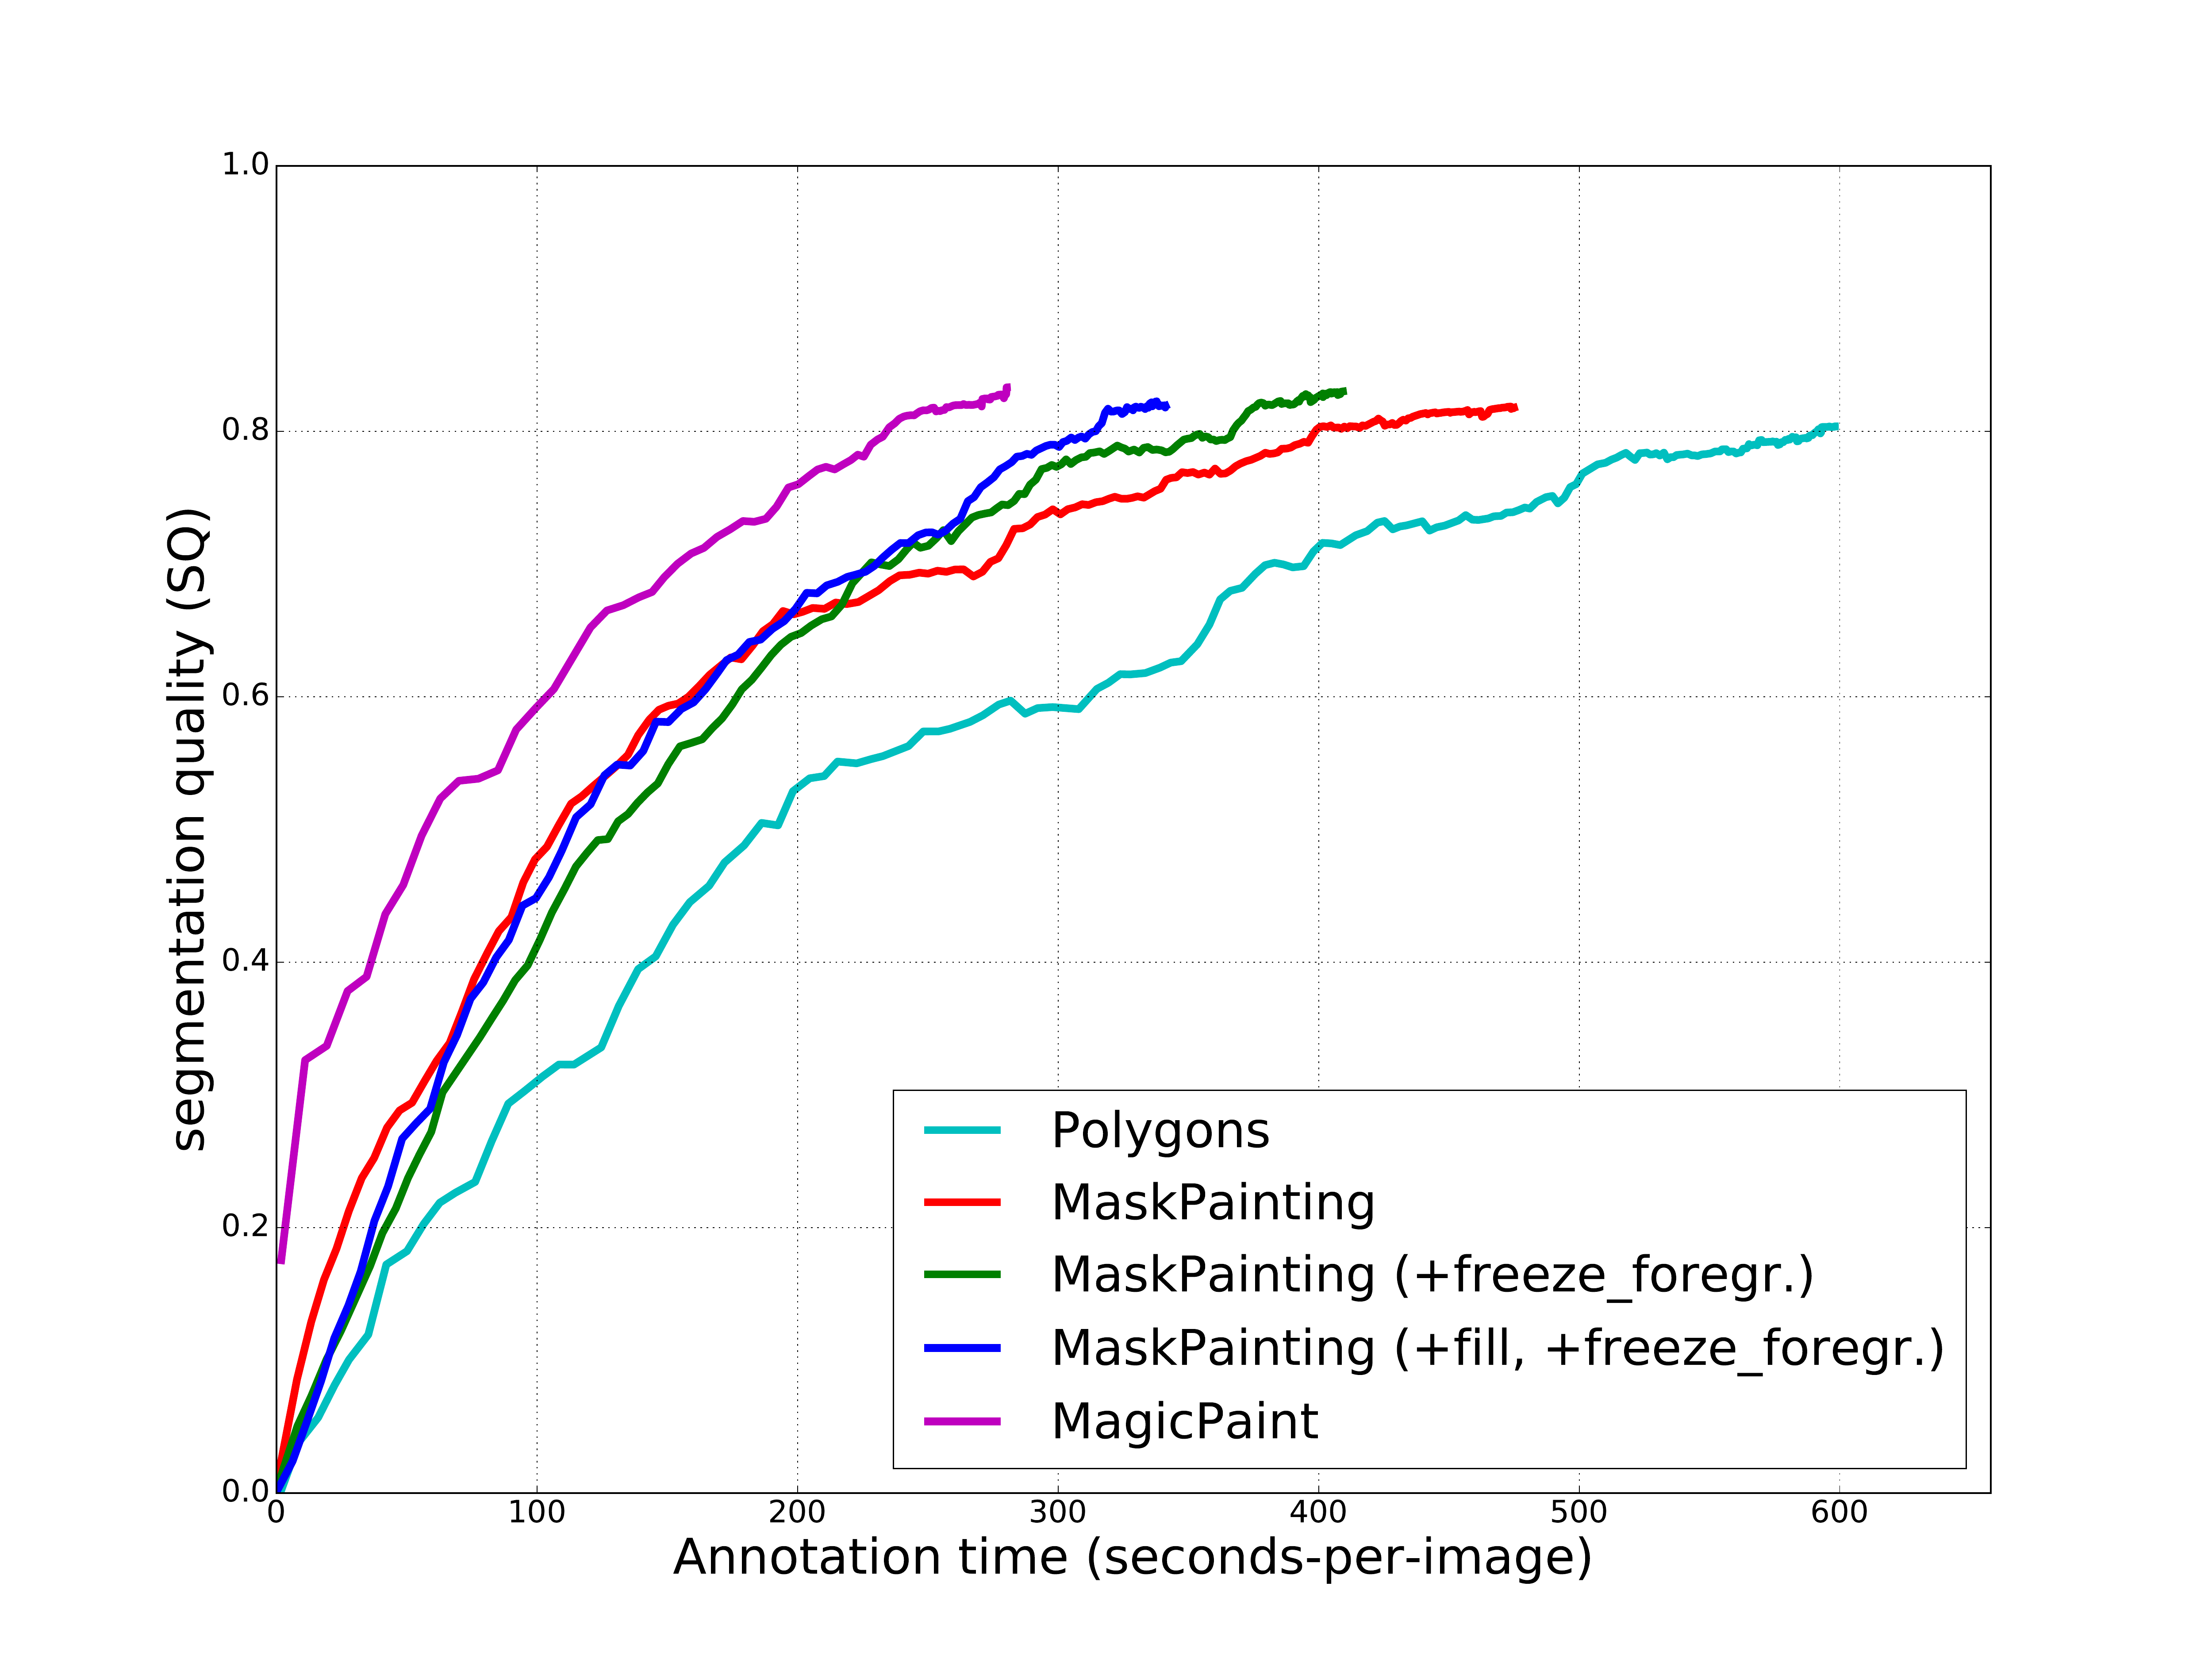}&
  \includegraphics[width=0.33\linewidth]{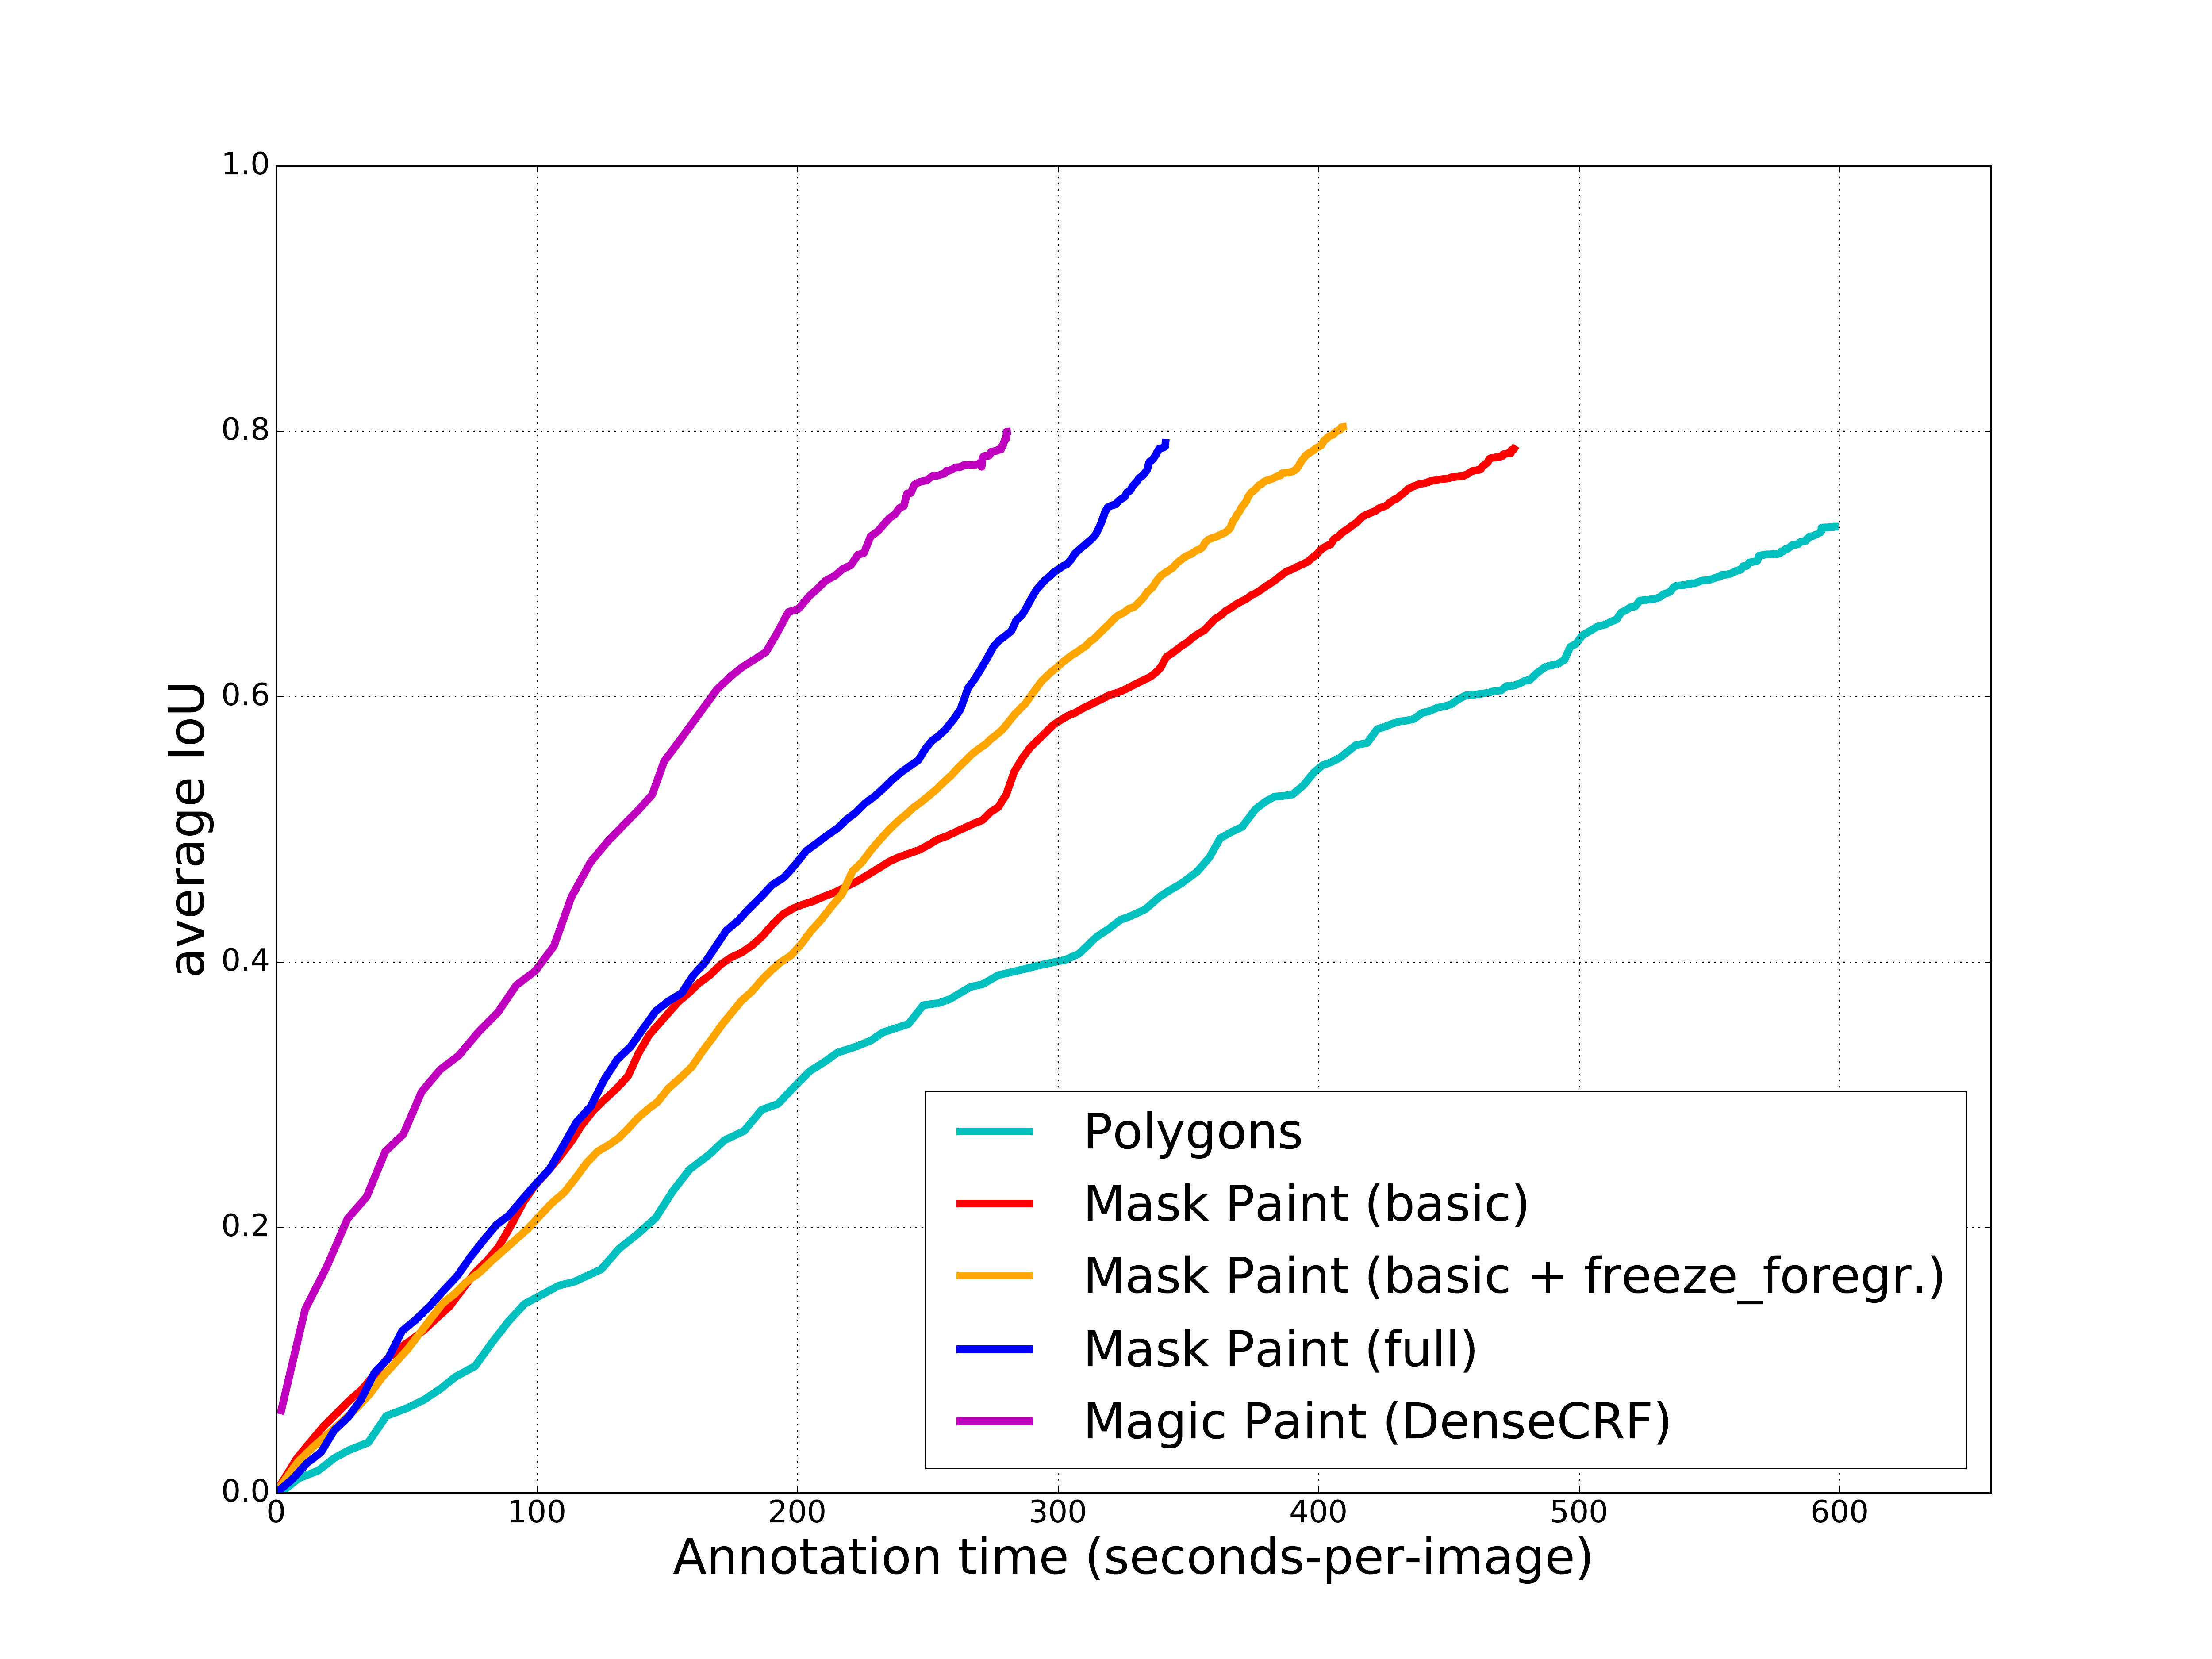}&
  \includegraphics[width=0.33\linewidth]{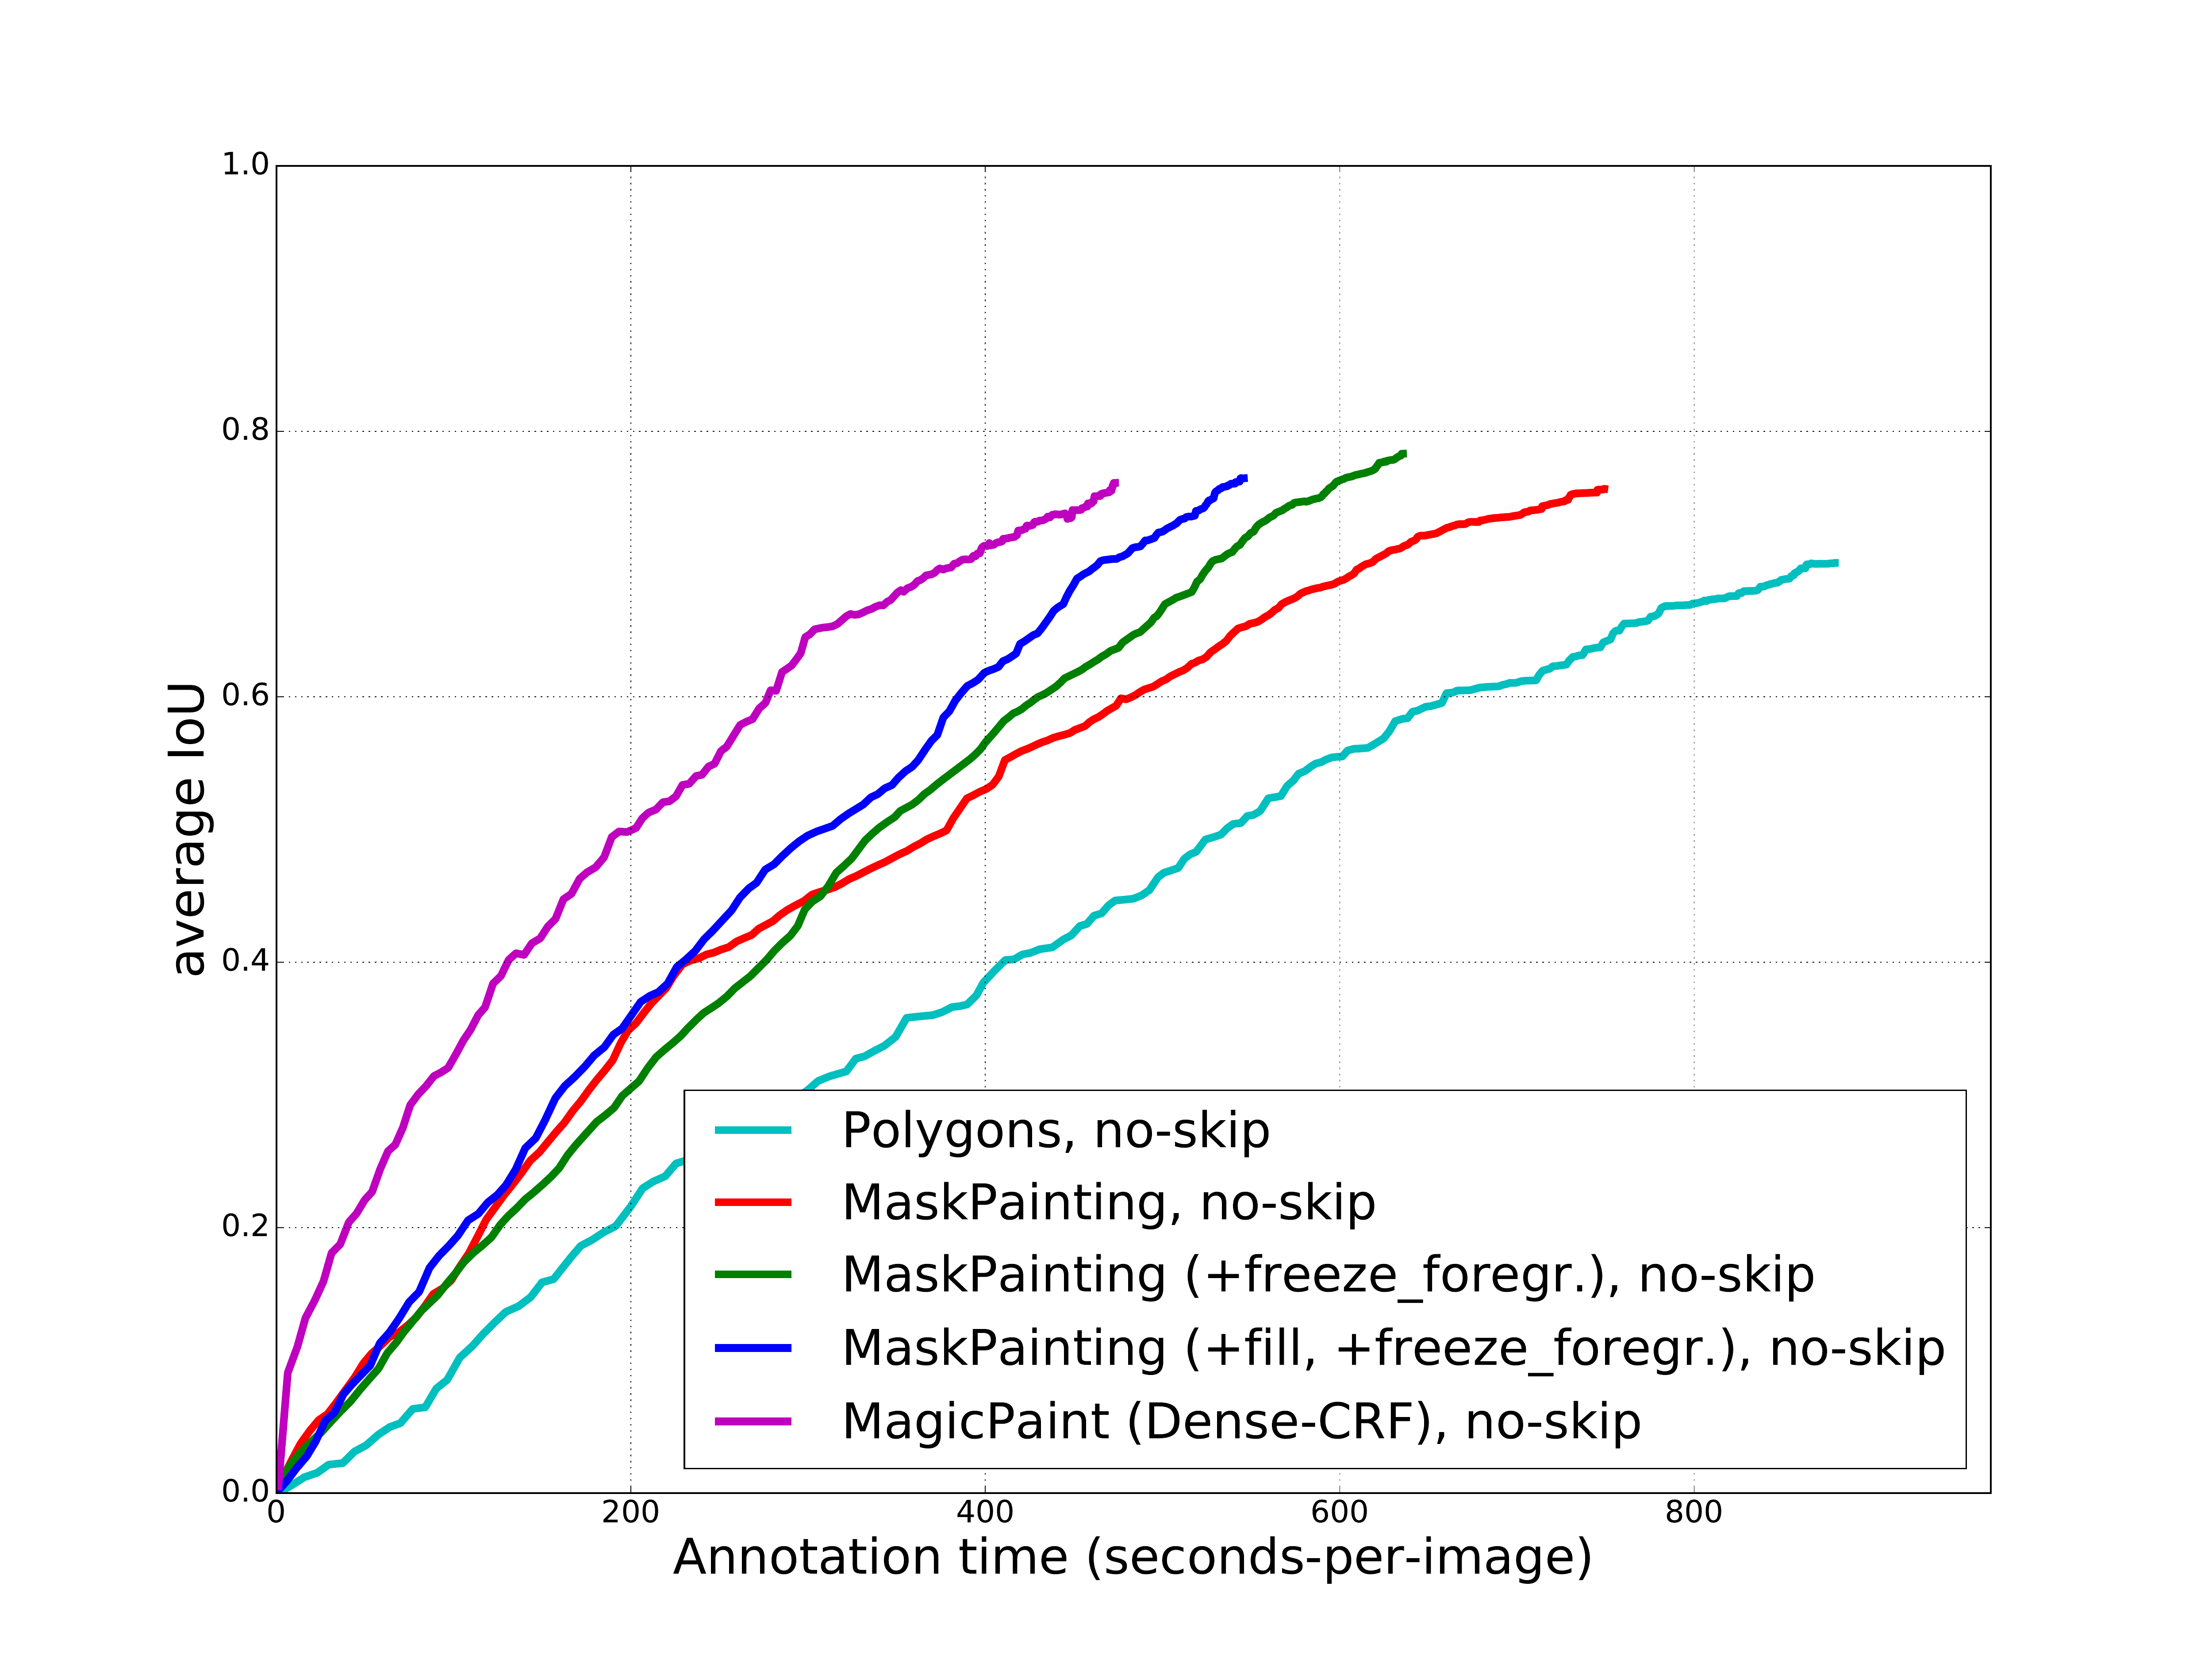}\\
(a) & (b) & (c)\\
\end{tabular}
\end{center}
\caption{Additional evaluation results on the COCO-val100 dataset. We compare evaluation results using segmentation quality (a) and average IoU (b). The plot in (c) shows evaluation without skipping redundant annotation actions. Note that the MagicPaint plots shown in (a) and (b) are the best-case plots that assume that predictions are available immediately.}
\label{fig:eval_appendix}
\end{figure}
